# Supplementary material for: Towards Stable Radial Basis Function Methods for Linear Advection Problems
Source: arXiv:2101.09623 source file (2021-01-24)
Supplement: Supplementary file 1 [file appendix.tex]

\section*{Appendix: }
\label{sec:appendix}
